# Supplementary material for: CryptoGuard: High Precision Detection of Cryptographic Vulnerabilities in Massive-sized Java Projects
Source: arXiv:1806.06881 source file (2019-03-27)
Supplement: Supplementary file 1 [file appendix1.tex]

\section*{Appendix A: Inter-procedural Backward Program Slicing}\label{appendix:a}

Here, we discuss different sub procedures of inter procedural backward program slicing Presented in Section~\ref{sec:inter-procedural-bs} in more details.

\begin{algorithm*}[h]
\caption{\textbf{\textit{calcInterProceduralSlices}} function in Algorithm~\ref{code:inter-procedural}.}
\label{code:sub-procedure}
\footnotesize
\begin{algorithmic}[1]
\Statex \textbf{Input:} \texttt{criterion, methodVsAnalysisMap, criteriaMap}
\Statex \textbf{Output:} \texttt{methodVsAnalysisMap}
\State \texttt{calsite} $\leftarrow$ \texttt{criterion.getCallsite()}
\State \texttt{slicingParams} $\leftarrow$ \texttt{criterion.getSlicingParams()}
\State \texttt{currMethod} $\leftarrow$ \texttt{callsite.getCaller()}

\If {\texttt{slicingParams} is empty $||$ \texttt{criteriaMap.get(criterion)} $!=$ null}
\Return
\EndIf

\State \texttt{criteriaMap.put(slicingCriteria, Boolean.TRUE)}
\State \texttt{prevAnalysis} $\leftarrow$ \texttt{methodVsAnalysisMap.get(callsite.getCallee())}
\State \texttt{currAnalysis} $\leftarrow$ \texttt{\textbf{calcIntraProceduralSlice}(currMethod, criterion)}
\If{\texttt{currAnalysis.getUsedFields()} is not empty}
\For{\texttt{field} in \texttt{currAnalysis.getUsedFields()}}
\State \texttt{listOfFieldSlicingResult} $\leftarrow$ \texttt{\textbf{calcSlicesForField}(field)}
\For{\texttt{fieldSlicingResult} in \texttt{listOfFieldSlicingResult}}
\State \texttt{containingMethod} $\leftarrow$ \texttt{fieldSlicingResult.getContainingMethod()}

\State \texttt{\textbf{storeAnalysisResult}(containingMethod, fieldSlicingResult, currAnalysis, prevAnalysis, methodVsAnalysisMap)}
\State \texttt{callers} $\leftarrow$ \texttt{containingMethod.getCallers()}
\State \texttt{callerSites} $\leftarrow$ \texttt{getCallsites(containingMethod, callers)}
\State \texttt{newParams} $\leftarrow$ \texttt{fieldSlicingResult.getInfluencingParams()}
\For{\texttt{newCallsite} in \texttt{callerSites}}
\State \texttt{newCriterion} $\leftarrow$ \texttt{new Criterion(newCallsite, newParams)}
\State \texttt{\textbf{calcInterProceduralSlices}(newCriterion, methodVsAnalysisMap, criteriaMap)}
\EndFor
\EndFor
\EndFor
\EndIf

\State \texttt{\textbf{storeAnalysisResult}(currMethod, currAnalysis, prevAnalysis, methodVsAnalysisMap)}
\State \texttt{callers} $\leftarrow$ \texttt{currMethod.getCallers()}
\State \texttt{callerSites} $\leftarrow$ \texttt{getCallsites(currMethod, callers)}
\State \texttt{newParams} $\leftarrow$ \texttt{currAnalysis.getInfluencingParams()}
\For{\texttt{newCallsite} in \texttt{callerSites}}
\State \texttt{newCriterion} $\leftarrow$ \texttt{new Criterion(newCallsite, newParams)}
\State \texttt{\textbf{calcInterProceduralSlices}(newCriterion, methodVsAnalysisMap, criteriaMap)}
\EndFor

\end{algorithmic}
\end{algorithm*} 

\paragraph{\texttt{buildCallerCalleeRelation} procedure.} 

Given a list of class names of a program, it builds the caller-callee relationship. If a method $m$ from a class $C_{1}$ invokes another method $m'$ from a class $C_{2}$ then we refer $m$ as the caller method and $m'$ as the callee method. If $m'$ is defined as a non-static method of $C_{2}$ then $m'$ can be overridden by any of its subclasses. The reference of $C_2$ can be used to access any such overridden version of $m'$. To avoid unsoundness we employ class hierarchy analysis~\cite{DBLP:conf/ecoop/DeanGC95} to consider all the overridden version of a method. However, considering all the versions are also known to cause numerous false positives. To trade-off between soundness and the false positives we only consider the direct subclasses.

In each method, we store all the references of its caller methods as a list, along with the list of call-site information of all the callee methods of it.

\paragraph{\texttt{calcInterProceduralSlices} procedure.}

Given a slicing criterion, the purpose of \texttt{calcInterProceduralSlices} is to calculate and store all the inter procedural slices by following the caller chain of the method recursively.
In Algorithm~\ref{code:sub-procedure}, we show the pseudo-code of our \texttt{calcInterProceduralSlices} procedure. At any point if we already did not collect the slices for a slicing criterion $criterion$ for a method $currMethod$ we proceed. First, we collect the intra procedural slice of $currMethod$ by invoking \texttt{calcIntraProceduralSlice} procedure with the corresponding slicing criterion (Line $10$). The \texttt{calcIntraProceduralSlice} returns the list of instructions that directly or indirectly influence the criterion. The result of \texttt{calcIntraProceduralSlice} also contains the information about the parameters of method $currMethod$ and also the fields that might directly or indirectly influence the criterion. After that it stores the slicing result (Line $28$). Then it follows the caller chain recursively (lines $29$ to $35$) to climb up the chain to find out all the influences till the top level caller methods. At any given method $currMethod$, it keeps track of the direction of the influence by storing the current slicing result ($currAnalysis$) and previous slicing results of the callee chain ($prevAnalysis$). The callee chain contains the previous results of all the slices that can lead to the original slicing criterion of interest. To achieve better soundness of the analysis, we also consider the influences of fields and their initializations (lines $12$ to $27$). For each of the influencing fields it finds their initializations by invoking \texttt{calcSlicesForField} (Line 14). \texttt{calcSlicesForField} returns the slices corresponding to the initialization instructions for a field together with the methods containing that initializations. Since, the field initializations from $containingMethod$ influence our slicing criterion in $currMethod$, to keep track of the direction of influence we store the current ($currAnalysis$), previous slicing results ($prevAnalysis$)  with the field slicing results ($fieldSlicingResult$). Then like previously, it also follows the caller chain recursively.

\paragraph{\texttt{calcSlicesForField} procedure.}

This is also a backward intra-procedural slicing mechanism. The specialty of this procedure is the type of the slicing criterion. Here, assign statements are considered as the slicing criterion. Here, we use assign statements for fields to calculate influencing instructions for it.

\paragraph{\texttt{storeAnalysisResult} procedure.}

This procedure creates and stores the analysis results for a method (first parameter). It stitches the analysis results. Specifically, it appends second parameter to the second last parameter by preserving the order and stores the result in the $methodVsAnalysisMap$ variable.
