# Supplementary material for: CryptoGuard: High Precision Detection of Cryptographic Vulnerabilities in Massive-sized Java Projects
Source: arXiv:1806.06881 source file (2019-03-27)
Supplement: Supplementary file 2 [file appendix2.tex]

\section*{Appendix B: Security Rules} \label{appendix:b}

\input{endpoints}

In this section we present the implementation details of the rule checkers. As we see in Table~\ref{table:rules}, the implementation of all of the rules requires various types program slicing. %In Table~\ref{tab:slicing-criteria} of Appendix~\ref{appendix:a} we present the slicing criteria corresponding to the rules.

\emph{Rules to detect whitebox secrets.} 

We use inter-procedural backward program slicing to find the predictable/constant values that is used as the keys for symmetric cryptography (Rule 1) and passwords for PBE (Rule 2) or cryptographic key stores (Rule 3). After finding the slices we find all the constants and the use of timestamps in that slices. After that we apply all the heuristics discussed in Section~\ref{impl:heuristics} to discard the pseudo-influencing candidates. The slicing criteria corresponding to each of the rules are presented in Table~\ref{tab:inter-slicing-criteria}.

\emph{Rules to detect MITM attacks on SSL/TLS.} 

In Rule 4, we find Hostname verifiers that accept all hosts. we look for all the classes that implements \texttt{HostnameVerifier} interface. All such classes defines \texttt{verify} method of \texttt{HostnameVerifier}. Using the \texttt{return} statement as the slicing criterion, we calculate intra-procedural backward slices of \texttt{verify} method. Ideally, such a slice should have the use of both the parameters of \texttt{verify} method. Any exception results in a warning.

In Rule 5, first we find all the implementation of \texttt{TrustManager}. Then we calculate intra-procedural backward slices for \texttt{checkServerTrusted} and \texttt{checkClientTrusted} by using \texttt{throw} as a slicing criterion. Also, we slice \texttt{getAcceptedIssuers} method by using \texttt{return} statement as the slicing criterion. 
An implementation of \texttt{TrustManager} should throw exceptions in \texttt{checkServerTrusted} and \texttt{checkClientTrusted} in the server or client certificate is not trusted. Also \texttt{getAcceptedIssuers} should return an array of certificates that would serve as the trust anchor. Any deviation from this is reported as a security violation. In Table~\ref{tab:methods-to-slice} we present the methods to slice and their corresponding slicing criteria for rules 4 and 5.

In Rule 6, if any method uses the slicing criteria specified in Table~\ref{tab:forward-slicing-criteria} to get an instance of a \texttt{SocketFactory}, then we perform a forward-program slicing of the method to find all the instructions that is influenced by the \texttt{SocketFactory} instance. After that we check the instructions from the slice to find any creation of socket that is not used as the parameter of the \texttt{verify} method of a \texttt{HostnameVerifier}.

In Rule 7, we calculate inter-procedural backward program slices to find the addresses that are used to create URLs to communicate with remote servers. The slicing criteria, we use for this purpose are specified in Appendix B. After that, if any address is found that uses HTTP protocol, we generate a warning.

\emph{Rules to detect insecure use of PRNGs.}
In Rule 8, we only consider the seeds of \texttt{SecureRandom}. We perform the inter-procedural program slices using the criteria presented in Appendix ~\ref{tab:inter-slicing-criteria}. We only consider \texttt{getSeed} or \texttt{generateSeed} method of \texttt{SecureRandom} as the safe source any deviation from this results in a warning. In Rule 9, we report any instantiation of \texttt{java.util.Random}.

\emph{Rules to prevent birthday attacks.}
For rules 10, 11, 12 first we perform inter-procedural backward program slicing with the respective slicing criteria presented in Table~\ref{tab:inter-slicing-criteria}. For rules 10 and 12, we apply heuristics to discard pseudo-influences. For Rule 11 we generate report if we find (1) the usage of AES with default mode (ECB is used by default) and (2) the usage of AES with ECB mode in the inter-procedural slices.

\emph{Rules to prevent bruteforce attacks.}
For Rule 13, 14, 16 we also perform inter-procedural backward program slicing. The corresponding slicing criteria is mentioned in Table~\ref{tab:inter-slicing-criteria}. After that for Rule 13 we look for integer constants that is less than $1000$ in each of the slices and report if we encounter one. For rules 14 and 16 we look for the insecure symmetric cryptographic primitives or hash functions in the slices as mentioned in Table~\ref{table:rules}. For Rule 15, we consider two cases (1) use of default size for RSA (2) setting key size explicitly. After creating an instance of RSA, if key size is not set by \texttt{initialize} method then we consider that this is using the default size (1024 bit). We use intra-procedural forward program slicing to find and report such cases where the slicing criteria is specified in Table~\ref{tab:forward-slicing-criteria}. We use inter-procedural backward program slicing to find key size if that is set explicitly.
